# Supplementary material for: Bias-Aware Sketches
Source: arXiv:1610.07718 source file (2017-03-26)
Supplement: Supplementary file 1 [file appendix.tex]

\section{A Comparison of Count-Median and Count-Min}
\label{sec:cm-exp}

The only difference between Count-Median and Count-Min is that in Count-Min, $\hat{x}_j$ is set to be $\min_{i\in[d]}  \left(\Pi(h^i)\bx\right)_{h^i(j)}$ instead of median (compared with Theorem~\ref{thm:count-median}). The theoretical error guarantees of the two algorithms are asymptotically the same, but Count-Min can only be used to handle non-negative vectors $\bx$. As indicated by \cite{CM04}, Count-Median can be thought as a generalization of Count-Min.   

Figure~\ref{fig:cm-cmn} gives a comparison between the Count-Median algorithm and the Count-Min algorithm, on datasets {\tt Yahoo}, {\tt Wiki} and {\tt Hudong}.  It can be seen that their performance in terms of average and maximum recovery errors is very close.

\begin{figure*}[t]
     \centering
     \subfloat[][{\tt Yahoo} Average Error]{\includegraphics[width=0.25\textwidth]{yahoo-cmn-ave}\label{fig:yahoo-cmn-ave}}
     \subfloat[][{\tt Yahoo} Maximum Error]{\includegraphics[width=0.25\textwidth]{yahoo-cmn-max}\label{fig:yahoo-cmn-max}}
     \subfloat[][{\tt Wiki} Average Error]{\includegraphics[width=0.25\textwidth]{wiki-cmn-ave}\label{fig:wiki-cmn-ave}}\\
     \subfloat[][{\tt Wiki} Maximum Error]{\includegraphics[width=0.25\textwidth]{wiki-cmn-max}\label{fig:wiki-cmn-max}}
     \subfloat[][{\tt Hudong} Average Error]{\includegraphics[width=0.25\textwidth]{hudong-cmn-ave}\label{fig:hudong-cmn-ave}}
     \subfloat[][{\tt Hudong} Maximum Error]{\includegraphics[width=0.25\textwidth]{hudong-cmn-max}\label{fig:hudong-cmn-max}}
     \caption{Count-Median versus Count-Min in {\tt Yahoo}, {\tt Wiki} and {\tt Hudong}}
     \label{fig:cm-cmn}
\end{figure*}
